# Supplementary material for: Solid Solubility in Metallic Hydrogen
Source: arXiv:2410.20762 source file (2024-10-28)
Supplement: Supplementary file 1 [file Supplementary_Materials.pdf]

# Supplemental Materials of Solid Solubility in Metallic Hydrogen.

**J Seeyangnok[1], U Pinsook[1], GJ Ackland[2]**

[1]Department of Physics, Faculty of Science, Chulalongkorn University, Bangkok, Thailand.

[2]Centre for Science at Extreme Conditions, School of Physics and Astronomy, University of Edinburgh, Edinburgh, United Kingdom.

E-mail: jakkapatjtp@gmail.com, Udomsilp.P@Chula.ac.th, gjackland@ed.ac.uk

October 2024

## Methods

In this work, we used the density functional theory (DFT) [1, 2] implemented in both Quantum Espresso (QE) [3, 4] and the CAmbridge Serial Total Energy Package (CASTEP) [5]. For ab initio molecular dynamics (AIMD), we used the AIMD implemented in CASTEP. Using the Broyden–Fletcher–Goldfarb–Shanno algorithm (BFGS) method [6–8], the $I4_1/amd$ structure of atomic metallic hydrogen, the BCC structure of beryllium (Be), magnesium (Mg), and sulfur (S), alpha-Gallium structure of Boron, the HPC structure of iron (Fe) , and the $I4/mmm$ structure of lanthanum (La) were fully optimized, employing a force convergence criterion of $1.0^{-5}$ eV/Å and a very dense Monkhorst-Pack grid k mesh to achieve a target pressure of 500 GPa. Pseudopotentials were modeled using the general gradient energy functional of Perdew–Burke–Ernzerhof (GGA-PBE) [9]. In Born-Oppenheimer molecular dynamics (BOMD) simulations, supercells of primitive cell structures were used, with a time step interval of 0.5 fs and integration was handled using the Verlet method [10]. The isothermal–isobaric ensemble (NPT) [11] was implemented, employing the Parrinello-Rahman barostat method [12] to maintain a pressure of 500 GPa. In addition, a thermostat was set at 300 K and equilibration was achieved using the Berendsen method [13]. The phonon density of states (PDOS) [14–17] was computed by performing a Fourier transformation of the velocity autocorrelation from the trajectory of each atom in AIMD given by,

$$g(\omega) = Re\left[\int e^{i\omega t}\frac{\langle \boldsymbol{v}(t)\cdot\boldsymbol{v}(0)\rangle}{\langle \boldsymbol{v}(0)\cdot\boldsymbol{v}(0)\rangle}dt\right]. \quad (1)$$

To analyze the results, we consider that the radial distribution function (RDF) can be calculated using the number density $\rho$ and

$$g(r) = \frac{1}{4\pi r^2 N\rho} \sum_{i=1}^{N} \sum_{k \neq i} \langle \delta(r + r_k - r_i) \rangle \,, \tag{2}$$

The mean squared displacement (MSD) can be computed using the ensemble average given by

$$MSD(t) = \left\langle |\boldsymbol{x}(t) - \boldsymbol{x}(0)|^2 \right\rangle . \tag{3}$$

We compute the phonon density of states (PhDOS) by performing a Fourier transformation of the velocity autocorrelation, [14–17], from the trajectory of each atom in AIMD given by,

$$D(\omega) = \int e^{i\omega t} \frac{\langle \boldsymbol{v}(t) \cdot \boldsymbol{v}(0) \rangle}{\langle \boldsymbol{v}(0) \cdot \boldsymbol{v}(0) \rangle} dt, \tag{4}$$

where the velocity autocorrelation (VAC) can be obtained using

$$VAC(t) = \langle \boldsymbol{v}(t) \cdot \boldsymbol{v}(0) \rangle \,. \tag{5}$$

with the time averaging over a sliding window for $t = 0$.

In order to check the reliability of the method, we computed the phonon spectrum of the pure $I4_1/amd$ metallic hydrogen structure at 500GPa using lattice dynamics and QE. In this case, the optimization of the structures was first obtained using the BFGS method [6, 7] by fully relaxing the crystal structures with the force of $1.0^{-5}$ eV/Å using the Monkhorst-Pack grid k mesh [18] of the $48 \times 48 \times 48$ k-point grid with Marzari-Vanderbilt-DeVita-Payne cold smearing of 0.02 Ry on the Fermi surface [19]. The optimized norm-conserving Vanderbilt pseudopotentials [20, 21] and the general gradient energy functional of the Perdew–Burke–Ernzerhof (GGA-PBE) [9] were implemented for the exchange correlation energy functional with wavefunction and charge density cutoffs of 120 Ry and 480 Ry, respectively. The irreducible matrix elements were calculated using QE, based on the density functional perturbation theory (DFPT) [22] with $12 \times 12 \times 12$ q-mesh grids.

The solubility of a substance is contingent upon the free energy it possesses, as expressed by the equation:

$$G = U + PV - TS$$

In our molecular dynamics (MD) simulations, we directly calculate the ensemble-averaged enthalpy $U + PV$, accounting for the kinetic energy and the thermal variation in the potential energy. However, determining the entropy $S$ is more complicated. Three elements contribute to the free energy but are not calculated directly: configurational entropy $S_{conf}$, zero-point energy of vibrations $U_{ZPE}$, and vibration entropy $S_{vib}$. The configurational entropy is represented in terms of the atomic fraction of the solute, $c$, as

$$S_{conf} = -k_b[c \ln(c) + (1 - c) \ln(1 - c)]$$

The zero-point energy of vibrations and entropy of vibrations are computed utilizing the phonon density of states under the harmonic approximation:

$$U_{ZPE} = \sum_{\mathbf{k},i} \frac{1}{2}\hbar\omega_{\mathbf{k},i}(V)$$

$$S_{vib} = -\sum_{\mathbf{k},i} k_B \ln\left[1 - \exp(-\hbar\omega_{\mathbf{k},i}(V)/k_B T)\right] + \frac{1}{T}\sum_{\mathbf{k},i} \frac{\hbar\omega_{\mathbf{k},i}(V)}{\exp(\hbar\omega_{\mathbf{k},i}(V)/k_B T) - 1}$$

The summation encompasses all frequencies in the lattice dynamics and may be replaced by a properly normalized integral over the probability distribution of the phonon density of states (PDOS), which we can obtain from the VAC of the molecular dynamics.

The determination of solubility limit would require identifying other compounds residing on the quasi-convex hull of the free energy. For a system with multiple components, extensive exploration within the composition space is required to ascertain the solute's chemical potential. This was beyond the scope of the present study, and turned out to be unnecessary for practical purposes because the negative free energy of the solution indicates the solute's solubility in metallic hydrogen or the formation of some hydride compound. Considering pure elements as the reference state, we can compute the free energy of solution by introducing one impurity (element $X$) and $N$ hydrogen atoms:

$$\Delta g_{sol} = g(X + NH) - g(X) - Ng(H) \tag{6}$$

The specific Gibbs free energies $g$ are evaluated in eV/impurity. Negative values indicate solubility in hydrogen, while positive values indicate finite solubility.

## RDF and MSD of substitutional alloys

The radial distribution function (RDF) and the mean square distance are shown (MSD) in Figures 1 for all substitutional alloys. RDF is computed using Eqn. 2, while MSD is calculated using Eqn. 3.

## Velocity autocorrelation of substitutional alloys

The velocity autocorrelation of substitutional alloys is computed using Eqn. 5 and shown in Figures 2. From these VAC, we computed corresponding PhDOS for free energy calculations.

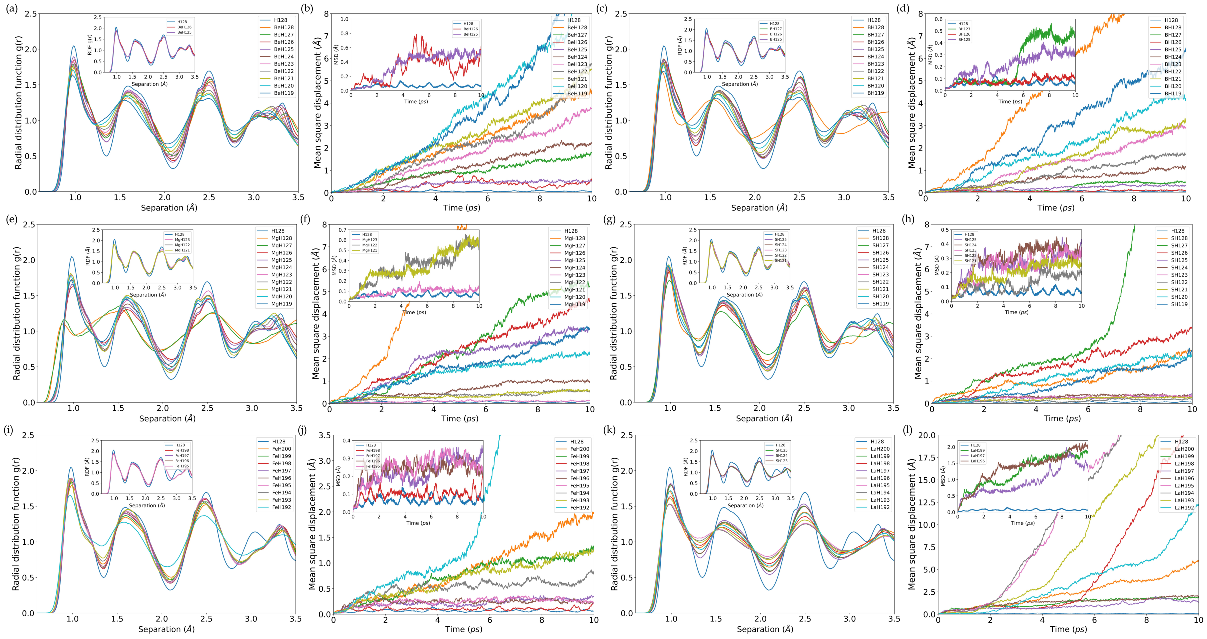


**Figure 1.** The figures show the radial distribution function and the mean square displacement of the substitutional alloys. (a-h) show the RDF and the MSD of $4 \times 4 \times 2$ supercell of substitutional alloys of Be, B, Mg, and S for different number of removing hydrogens. (i-l) display the RDF and the MSD of $5 \times 5 \times 2$ supercell of substitutional alloys consisting of Fe, and La for different number of removed hydrogens.

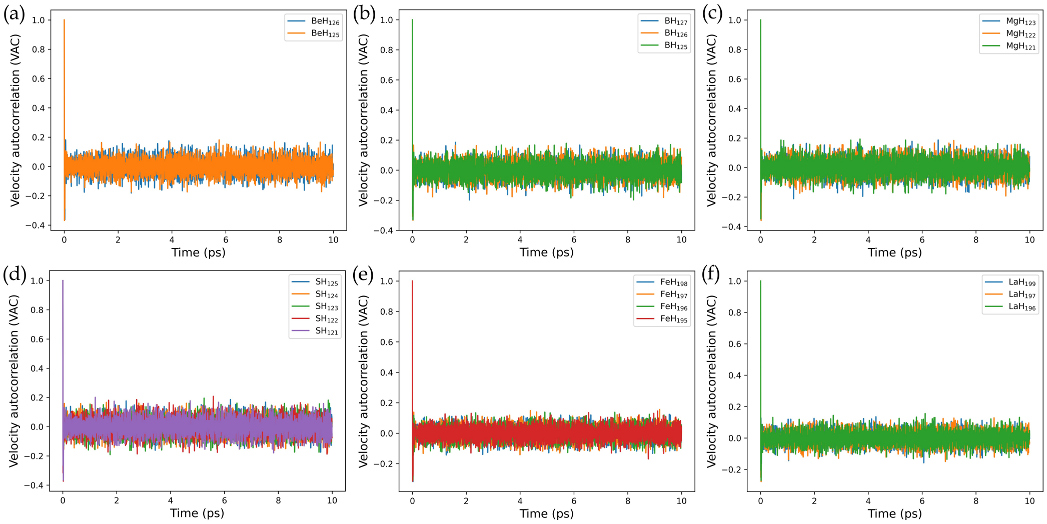


**Figure 2.** The figures show the good equilibration of the velocity autocorrelation of substitutional alloys.

## Phonon density of states of $I4_1/amd$ metallic hydrogen, alloys, and substitutional alloys.

The phonon density of states obtained from the MD and DFPT methods is shown in Figure 3 with blue (DFPT) and orange (MD) lines. Although there are some differences

in the phonon density of states between the two methods, the vibrational entropy ($TS$) and zero-point energy ($U_{ZPE}$) of both methods is very similar, as shown in Table 1. These results confirm that our methods for accounting for the vibrational contributions due to thermal effects via VAC are valid.

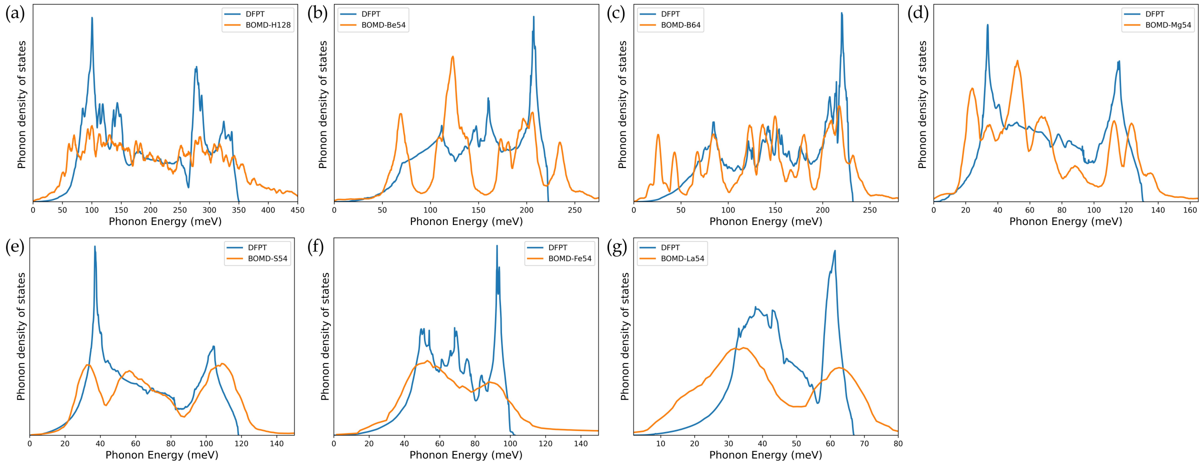


**Figure 3.** (a-d) Blue lines show the phonon density of state (PhDOS) from the DFT calculations based on the DFPT method computed from primitive structures of H, Be, B, and Mg, respectively. (a-d) Orange lines show PhDOS from BOMD at 500GPa and 300K with 128 hydrogen atoms, 54 berillium atoms, 64 boron atoms 54 magnesium atoms, 54 sulfur atoms, 54 iron atoms, and 54 lanthanum atoms, respectively.

| Alloys | $H$ | $TS_{MD}$ ($TS_{DFPT}$) | $U_{ZPE_{MD}}$ ($U_{ZPE_{DFPT}}$) | $G$ |
|---|---|---|---|---|
| H | -9.7595±0.0004 | 0.0050±0.0001 (0.0036) | 0.3309±0.0049 (0.2920) | -9.4336±0.0049 |
| Be | -378.1031±0.0004 | 0.0064±0.0009 (0.0050) | 0.2339±0.0061 (0.2230) | -377.8757±0.0062 |
| B | -76.8754±0.0006 | 0.0117±0.0004 (0.0058) | 0.2262±0.0031 (0.2284) | -76.6609±0.0032 |
| Mg | -1659.5462±0.0030 | 0.0352±0.0019 (0.0296) | 0.1094±0.0048 (0.1079) | -1659.4720±0.0060 |
| S | -276.3689±0.0018 | 0.0265±0.0029 (0.0325) | 0.1168±0.0044 (0.0977) | -276.2786±0.0056 |
| Fe | -839.4998±0.0019 | 0.0267±0.0026 (0.0256) | 0.1119±0.0054 (0.1019) | -839.4146±0.0062 |
| La | -923.1902±0.0009 | 0.0559±0.0058 (0.0465) | 0.0675±0.0087 (0.0680) | -923.1786±0.0105 |

**Table 1.** The table shows the enthalpies ($H$ (eV/atom)), the entropy consisting of both vibrational entropy and configurational entropy ($S = S_{vib} + S_{confi.}$ (eV/atom)), the zero-point energy of phonon ($U_{ZPE}$ (eV/atom)), and the Gibbs free energy $G$ (eV/atom).

The excessive decimal accuracy of ensemble values in Table 1 and Table 2 is limited to four decimal places when the unit is energy per atom, and two decimal places when the unit is energy per alloy, as presented in the paper. For static calculations such as entropy and zero-point energy from DFT calculations, we do not account for methodological errors, as the convergence of DFT energy calculations is accurate to many significant

figures. Therefore, the difference is not comparable to those ensemble values. Fig. 4 (a)-(f), we show the phonon density of states obtained from BOMD with methods explained previously.

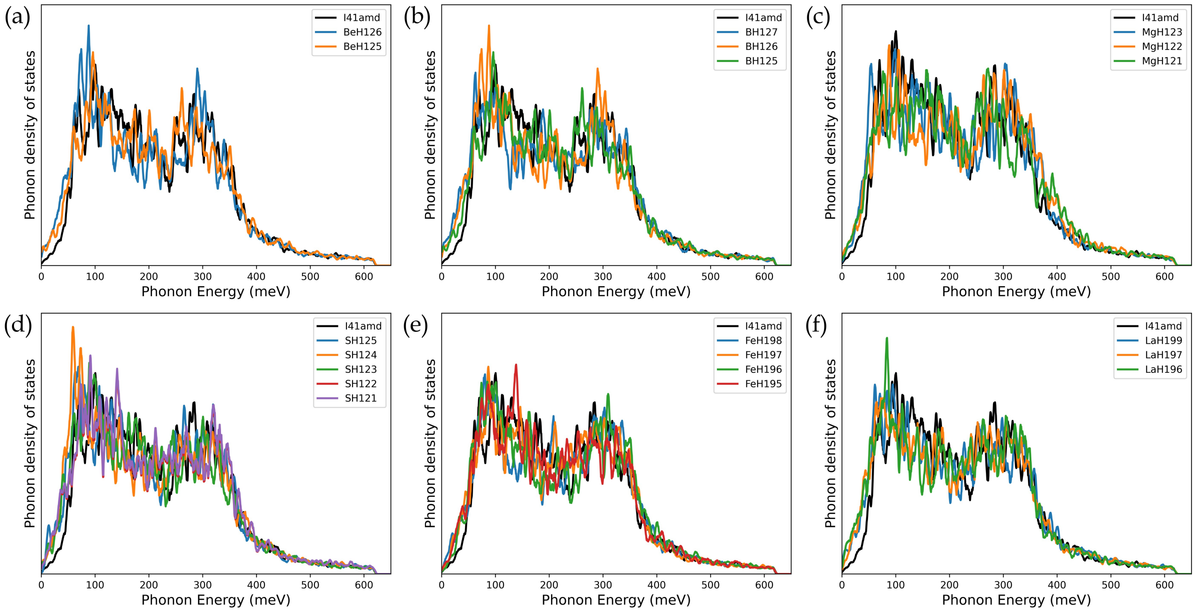


**Figure 4.** (a-f) show the phonon density of states obtained from BOMD of structures of substitutional alloys discussed in the paper where we also plot PhDOS of $I4_1/amd$ of metallic hydrogen.

## Structures of substitutional alloys.

The structures of substitutional alloys of neighbouring hydrogens is considered through the radial distribution function of hydrogen with respect to alloys as shown in Figures 5 showing the significant first peak of neighbouring hydrogens. The number of hydrogens sorrounding alloys is considered using the cumulative number of pairs (CDF) between alloy and hydrogens as shown in Figures 6.

## Free energies of $I4_1/amd$ metallic hydrogen, alloys and substitutional alloys.

The enthalpy presented in Table 2 is the average value of the MD simulations, including the associated uncertainty. To account for the uncertainty in the vibrational entropy ($TS_{\text{vib}}$) and the zero-point energy ($U_{\text{ZPE}}$), we divide the VAC into four equally independent samples ($\text{VAC}^1$, $\text{VAC}^2$, $\text{VAC}^3$, and $\text{VAC}^4$). From these four samples, we compute four independent values of the vibrational entropy ($TS^1_{\text{vib}}$, $TS^2_{\text{vib}}$, $TS^3_{\text{vib}}$, and $TS^4_{\text{vib}}$) and the zero-point energy ($U^1_{\text{ZPE}}$, $U^2_{\text{ZPE}}$, $U^3_{\text{ZPE}}$, and $U^4_{\text{ZPE}}$). Then, we define the uncertainty of the vibrational entropy and the uncertainty of the zero-point energy using

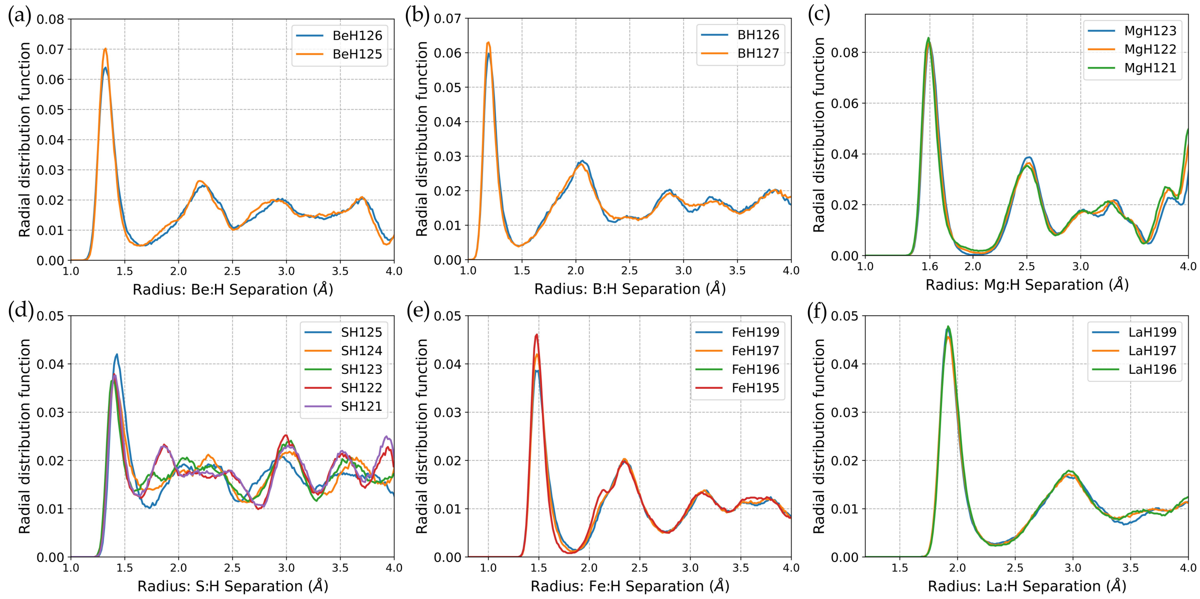


**Figure 5.** (a-f) shows the radial distribution function (RDF) of alloy-hydrogen pair distribution at certain distance of structures of substitutional alloys discussed in the paper.

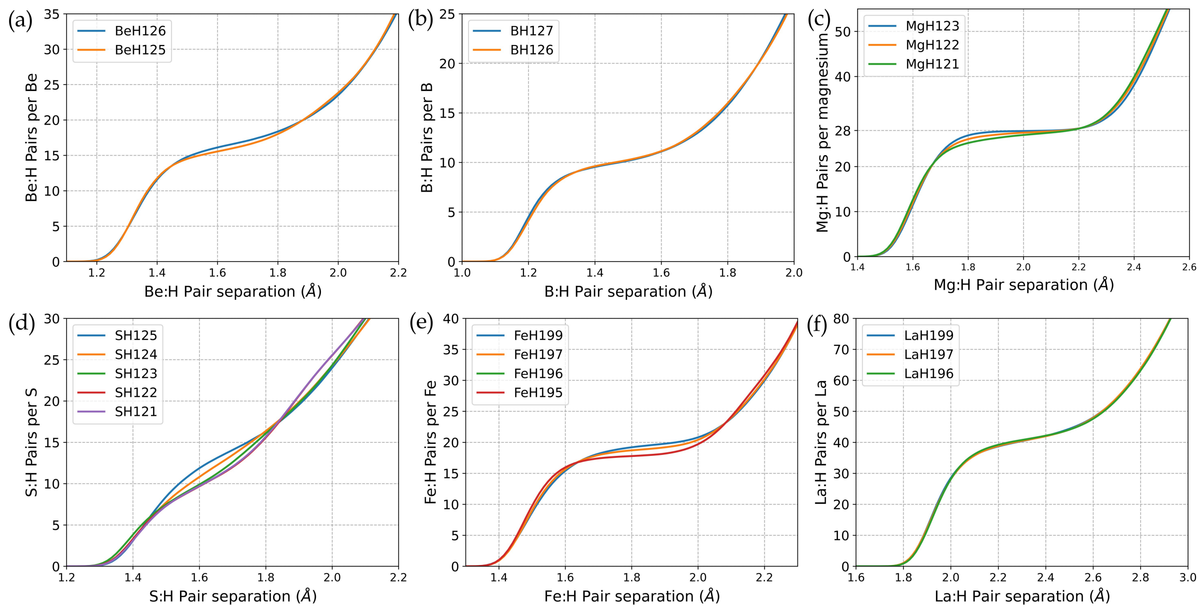


**Figure 6.** (a-f) shows the cumulative number of pairs between alloy and hydrogens at certain distance of structures of substitutional alloys discussed in the paper.

the standard deviation, $\sigma = \sqrt{\frac{\sum_{i=1}^{4}(x_i - \mu)^2}{4}}$ where $x_i$ and $\mu$ are the four values, and the average value, respectively. Driving down this uncertainty is crucial because in the energy differences per impurity (Table I, main paper) they will be multiplied by the

number of atoms. The statistical errors are similar to the effect of anharmonicity as shown in Table 1 where we can perform DFPT calculations and compare the results to those obtained from MD simulations. In this analysis, we have chosen to calculate the error for each system independently: a case could be made for assuming the errors are the same for every VAC.

| $MH_x$ | $H$ | $TS$ | $U_{ZPE}$ | $G$ |
|---|---|---|---|---|
| $BeH_{126}$ | -12.6631±0.0006 | 0.0075±0.0004 | 0.3207±0.0048 | -12.3516±0.0049 |
| $BeH_{125}$ | -12.6867±0.0007 | 0.0067±0.0006 | 0.3258±0.0026 | -12.3694±0.0027 |
| $BH_{127}$ | -10.2714±0.0008 | 0.0070±0.0001 | 0.3188±0.0046 | -9.9612±0.0047 |
| $BH_{126}$ | -10.2760±0.0008 | 0.0069±0.0003 | 0.3174±0.0048 | -9.9672±0.0049 |
| $BH_{125}$ | -10.2814±0.0009 | 0.0065±0.0005 | 0.3264±0.0049 | -9.9633±0.0050 |
| $MgH_{123}$ | -23.1194±0.0006 | 0.0068±0.0003 | 0.3310±0.0060 | -22.7969±0.0060 |
| $MgH_{122}$ | -23.2282±0.0010 | 0.0064±0.0004 | 0.3421±0.0033 | -22.8942±0.0034 |
| $MgH_{121}$ | -23.3407±0.0008 | 0.0063±0.0005 | 0.3341±0.0067 | -23.0146±0.0068 |
| $SH_{125}$ | -11.8648±0.0008 | 0.0078±0.0006 | 0.3184±0.0042 | -11.5559±0.0043 |
| $SH_{124}$ | -11.8822±0.0009 | 0.0083±0.0007 | 0.3124±0.0064 | -11.5799±0.0065 |
| $SH_{123}$ | -11.9007±0.0006 | 0.0073±0.0005 | 0.3166±0.0073 | -11.5932±0.0073 |
| $SH_{122}$ | -11.9183±0.0006 | 0.0073±0.0002 | 0.3250±0.0052 | -11.6023±0.0052 |
| $SH_{121}$ | -11.9376±0.0009 | 0.0078±0.0005 | 0.3229±0.0017 | -11.6242±0.0020 |
| $FeH_{198}$ | -13.9330±0.0005 | 0.0067±0.0002 | 0.3320±0.0023 | -13.6090±0.0024 |
| $FeH_{197}$ | -13.9539±0.0006 | 0.0062±0.0005 | 0.3285±0.0073 | -13.6328±0.0074 |
| $FeH_{196}$ | -13.9761±0.0008 | 0.0064±0.0002 | 0.3305±0.0058 | -13.6532±0.0059 |
| $FeH_{195}$ | -13.9968±0.0005 | 0.0066±0.0002 | 0.3271±0.0057 | -13.6775±0.0058 |
| $LaH_{199}$ | -14.3317±0.0010 | 0.0077±0.0007 | 0.3262±0.0048 | -14.0144±0.0050 |
| $LaH_{197}$ | -14.3789±0.0005 | 0.0074±0.0008 | 0.3256±0.0063 | -14.0619±0.0063 |
| $LaH_{196}$ | -14.4015±0.0006 | 0.0081±0.0011 | 0.3242±0.0070 | -14.0866±0.0071 |

**Table 2.** The table shows the enthalpies ($H$ (eV/atom)), the entropy consisting of both vibrational entropy and configurational entropy ($S = S_{vib} + S_{confi.}$ (eV/atom)), the zero-point energy of phonon ($U_{ZPE}$ (eV/atom)), and the Gibbs free energy $G$ (eV/atom).

## References

[1] Hohenberg P and Kohn W 1964 *Phys. Rev.* **136** B864–B871
[2] Kohn W and Sham L J 1965 *Phys. Rev.* **140** A1133–A1138
[3] Giannozzi P, Baroni S, Bonini N, Calandra M, Car R, Cavazzoni C, Ceresoli D, Chiarotti G L, Cococcioni M, Dabo I *et al.* 2009 *Journal of physics: Condensed matter* **21** 395502
[4] Giannozzi P, Andreussi O, Brumme T, Bunau O, Nardelli M B, Calandra M, Car R, Cavazzoni C, Ceresoli D, Cococcioni M *et al.* 2017 *Journal of physics: Condensed matter* **29** 465901
[5] Clark S J, Segall M D, Pickard C J, Hasnip P J, Probert M J, Refson K and Payne M 2005 *Z. Kristall.* **220** 567–570
[6] Pfrommer B G, Cote M, Louie S G and Cohen M L 1997 *J. Comput. Phys.* **131** 233–240
[7] Liu D C and Nocedal J 1989 *Mathematical programming* **45** 503–528
[8] Payne M C, Teter M P, Allan D C, Arias T and Joannopoulos J D 1992 *Rev. Mod. Phys.* **64** 1045–1097
[9] Perdew J P, Burke K and Ernzerhof M 1996 *Physical review letters* **77** 3865
[10] Swope W C, Andersen H C, Berens P H and Wilson K R 1982 *J. Chem. Phys.* **76** 637–649
[11] Martyna G L, Klein M L and Tuckerman M 1992 *J. Chem. Phys.* **97** 2635–2645
[12] Parrinello M and Rahman A 1981 *J. Appl. Phys.* **52** 7182–7190
[13] Berendesen H J C, Postma J P M, Van Gunsteren W F, Di Nola A and Haak J 1984 *J. Chem. Phys.* **81** 2684–2690
[14] Dove M T 1993 *Introduction to lattice dynamics* 4 (Cambridge university press)
[15] Dickey J and Paskin A 1969 *Physical Review* **188** 1407
[16] Heino P 2007 *The European Physical Journal B* **60** 171–179
[17] Kong L T 2011 *Computer Physics Communications* **182** 2201–2207
[18] Monkhorst H J and Pack J D 1976 *Physical review B* **13** 5188
[19] Marzari N, Vanderbilt D, De Vita A and Payne M 1999 *Physical review letters* **82** 3296
[20] Hamann D 2013 *Physical Review B* **88** 085117
[21] Schlipf M and Gygi F 2015 *Computer Physics Communications* **196** 36–44
[22] Baroni S, De Gironcoli S, Dal Corso A and Giannozzi P 2001 *Reviews of modern Physics* **73** 515
